# Supplementary material for: Structured Knowledge Grounding for Question Answering
Source: arXiv:2209.08284 source file (2023-06-05)
Supplement: Supplementary file 1 [file 6-appendix.tex]

\appendix
\section{Hyperparameters}
\input{tables/tbl_hyperparameter}
